# Supplementary material for: Hybrid Random Features
Source: arXiv:2110.04367 source file (2022-01-30)
Supplement: Supplementary file 1 [file appendix.tex]

\section*{APPENDIX: Rethinking Softmax Approximation}

\subsection{Proof of Theorem \ref{reg-theorem}}
\begin{proof}
Let $\mathbf{x}, \mathbf{y} \in \mathbb{R}^{d}$ be respectively a query/key.
Note that from the definition of $\mathrm{SM}^{\mathrm{reg}}(\mathbf{x}, \mathbf{y})$ we have
for $\mathbf{z} = \mathbf{x}+\mathbf{y}$:
\begin{equation}
\mathrm{SM}^{\mathrm{reg}}(\mathbf{x}, \mathbf{y}) = 
\exp(-\frac{\|\mathbf{x}\|^{2}+\|\mathbf{y}\|^{2}}{2})
\sum_{k=0}^{\infty}\frac{1}{(2k)!}\|\mathbf{z}\|^{2k}d^{k}\mathbb{E}_{\omega \sim \mathcal{N}(0, \mathbf{I}_{d})}[(\frac{\omega}{\|\omega\|_{2}}\mathbf{e}_{1})^{2k}],
\end{equation}
where $\mathbf{e}_{1} \overset{\mathrm{def}}{=} (1,0,...,0)^{\top} \in \mathbb{R}^{d}$. To obtain the above we used the fact that $\mathcal{N}(0, \mathbf{I}_{d})$ is isotropic (that in particular implies zeroing of the even terms in the Taylor expansion).

Let us denote: $A(k, d) \overset{\mathrm{def}}{=} \mathbb{E}_{\omega \sim \mathcal{N}(0, \mathbf{I}_{d})}[(\frac{\omega}{\|\omega\|_{2}}\mathbf{e}_{1})^{2k}]$. It turns out that:
\begin{equation}
A(2k, d) = \frac{(2k-1)!!}{(d+2k-2)(d+2k-4) \cdot ... \cdot d}.    
\end{equation}
The proof of that fact can be found in the supplement of \cite{geometry}, yet we provide it below for completeness and the convenience of the Reader:
\begin{lemma}
Expression $A(2k, d)$ satisfies the following for $k \in \mathbb{N}$ :
\begin{equation}
A(2k, d) = \frac{(2k-1)!!}{(d+2k-2)(d+2k-4) \cdot ... \cdot d}.     
\end{equation}
\end{lemma}
\begin{proof}
Note first that for $d \geq 2$ the density function $p_{d}(\theta)$ of the angle between a vector $\mathbf{r} \in \mathbb{R}^{d}$ chosen uniformly at random from the unit sphere and $\mathbf{e}_{1}$ is given by the following formula:
\begin{equation}
p_{d}(\theta) = \frac{\sin^{d-2}(\theta)}{\int_{0}^{\pi}\sin^{d-2(\theta)}d\theta}.    
\end{equation}
Let us denote: $F(k, d) \overset{\mathrm{def}}{=} \int_{0}^{\pi}\cos^{k}(\theta)\sin^{d}(\theta)d\theta$.
Using partial integration, we get:
\begin{align}
\begin{split}
\int_{0}^{\pi}\cos^{k}(\theta)\sin^{d}(\theta)d\theta=
\int_{0}^{\pi}\cos^{k-1}(\theta)\sin^{d}(\theta)(\sin(\theta))^{\prime}d\theta= \\
\cos^{k-1}(\theta)\sin^{d+1}(\theta)|^{\pi}_{0} - 
\int_{0}^{\pi}\sin(\theta)
(
(k-1)\cos^{k-2}(\theta)(-\sin(\theta))\sin^{d}(\theta)+\\
d\cos^{k}(\theta)\sin^{d-1}(\theta)
)d\theta.
\end{split}
\end{align}
Thus we conclude that: $F(k, d) = \frac{k-1}{d+1}F(k-2, d+2)$.
Therefore we have: 
\begin{equation}
F(2k, d) = \frac{(2k-1)!!}{(d+1)(d+3)\cdot...\cdot(d+2k-1)}
\int_{0}^{\pi}\sin^{d+2k}(\theta) d\theta.
\end{equation}
We again conduct partial integration and get:
\begin{align}
\begin{split}
\int_{0}^{\pi}\sin^{d}(\theta)d\theta = -\frac{1}{d}\sin^{d-1}(\theta)\cos(\theta)|^{\pi}_{0} + \\
\frac{d-1}{d}\int_{0}^{\pi}\sin^{d-2}(\theta)d\theta = 
\frac{d-1}{d}\int_{0}^{\pi}\sin^{d-2}(\theta)d\theta.
\end{split}
\end{align}
Therefore we conclude that:
\begin{align}
\begin{split}
A(2k, d) = \frac{1}{\frac{d-3}{d-2}\frac{d-5}{d-4}\cdot ...}
\frac{(2k-1)!!}{(d-1)(d+1)\cdot...\cdot(d+2k-3)}
\frac{d+2k-3}{d+2k-2}\frac{d+2k-5}{d+2k-4} \cdot ....
= \\ \frac{(2k-1)!!}{(d+2k-2)(d+2k-4) \cdot ... \cdot d},
\end{split}
\end{align}
which completes the proof.
\end{proof}
Applying the above lemma, we get:
\begin{align}
\begin{split}
\mathrm{SM}^{\mathrm{reg}}(\mathbf{x}, \mathbf{y}) = 
\exp(-\frac{\|\mathbf{x}\|^{2}+\|\mathbf{y}\|^{2}}{2})
\sum_{k=0}^{\infty}\frac{1}{(2k)!}
\|\mathbf{z}\|^{2k}d^{k}\frac{(2k-1)!!}{(d+2k-2)(d+2k-4)\cdot...\cdot d} \\ = 
\exp(-\frac{\|\mathbf{x}\|^{2}+\|\mathbf{y}\|^{2}}{2})
\sum_{k=0}^{\infty} \frac{w^{k}}{k!}f(k, d),
\end{split}
\end{align}
where $w = \frac{\|\mathbf{z}\|^{2}}{2}$
and $f(k, d) = \frac{d^{k}}{(d+2k-2)(d+2k-4)\cdot...\cdot d}$.

Thus we obtain:
\begin{equation}
\frac{\mathrm{SM}^{\mathrm{reg}}(\mathbf{x}, \mathbf{y})}{\mathrm{SM}(\mathbf{x}, \mathbf{y})} = 
e^{-w}\sum_{k=0}^{\infty} \frac{w^{k}}{k!}f(k, d).
\end{equation}
Note first that for $k \geq 1$ we have: $f(k, d) \leq 1$, thus:
\begin{equation}
\mathrm{SM}^{\mathrm{reg}}(\mathbf{x}, \mathbf{y}) \leq \mathrm{SM}(\mathbf{x}, \mathbf{y}).    
\end{equation}
We also have for $l=d^{\frac{1}{3}}$:
\begin{align}
\begin{split}
\frac{\mathrm{SM}^{\mathrm{reg}}(\mathbf{x}, \mathbf{y})}{\mathrm{SM}(\mathbf{x}, \mathbf{y})} = 
e^{-w}\sum_{k=0}^{l} \frac{w^{k}}{k!}f(k, d) +  
e^{-w}\sum_{k=l+1}^{\infty} \frac{w^{k}}{k!}f(k, d) \geq \\
f(l, d) e^{-w}\sum_{k=0}^{l} \frac{w^{k}}{k!} +
e^{-w}\sum_{k=l+1}^{\infty} \frac{w^{k}}{k!}f(k, d) \geq
f(l, d)(1 - e^{-w}\sum_{k=l+1}^{\infty} \frac{w^{k}}{k!}) = \\
f(l, d)(1-\mathbb{P}[\mathrm{Po}(w) > l]),
\end{split}
\end{align}
where $\mathrm{Po}(w)$ stands for the random variable of Poisson distribution with parameter $w$.
Therefore we get for $t = \ln(\frac{l}{w})$:
\begin{align}
\begin{split}
\frac{\mathrm{SM}^{\mathrm{reg}}(\mathbf{x}, \mathbf{y})}{\mathrm{SM}(\mathbf{x}, \mathbf{y})} \geq 
(1-\frac{2l-2}{d})^{l}(1-\mathbb{P}[\mathrm{Po}(w) > l]) \geq \\
\exp(l \ln(1-\frac{2l-2}{d}))(1-\mathbb{P}[t\mathrm{Po}(w) \geq tl]) = \\
\exp\left(l \sum_{i=1}^{\infty}(-1)^{i}\frac{(\frac{2l-2}{d})^{i}}{i}\right)(1-\mathbb{P}[\exp(t\mathrm{Po}(w)-tl) \geq 1]) \geq \\
\exp(-\frac{2}{d^{\frac{1}{3}}}+o(\frac{1}{d^{\frac{1}{3}}}))
(1-\exp(-tl)\mathbb{E}[\exp(t\mathrm{Po}(w))])
= \\
\exp(-\frac{2}{d^{\frac{1}{3}}}+o(\frac{1}{d^{\frac{1}{3}}}))
(1-\exp(-w-l(t-1))),
\end{split} 
\end{align}
where the last equality is implied by the formula for the Laplace Transform for the Poisson random variable:
\begin{equation}
\mathbb{E}[\exp(t\mathrm{Po}(w))] = \exp(w(\exp(t)-1)).    
\end{equation}
Notice that: 
$w = \frac{\|\mathbf{z}\|^{2}}{2} = \frac{\ln(\mathrm{SM}(\mathbf{x},\mathbf{x}))+\ln(\mathrm{SM}(\mathbf{y},\mathbf{y})) + 2\ln(\mathrm{SM}(\mathbf{x}, \mathbf{y}))}{2} \leq 2\ln(C)$.
We conclude that:
\begin{equation}
\frac{\mathrm{SM}^{\mathrm{reg}}(\mathbf{x}, \mathbf{y})}{\mathrm{SM}(\mathbf{x}, \mathbf{y})} \geq  
(1-\frac{2}{d^{\frac{1}{3}}}+o(\frac{1}{d^{\frac{1}{3}}}))(1-C^{-2}(\frac{d^{\frac{1}{3}}}{2e \cdot \ln(C)})^{-d^{\frac{1}{3}}})
=1 - \frac{2}{d^{\frac{1}{3}}} + o(\frac{1}{d^{\frac{1}{3}}}).
\end{equation}
That completes the proof.
\end{proof}

\subsection{Proof of Lemma \ref{mse-lemma}}
\begin{proof}
Note that by using standard trigonometric identities (and the fact that the variance of the sum of independent random variables is the sum of variances of those random variables), we can get the following for $\omega \sim \mathcal{N}(0, \mathbf{I}_{d})$:
\begin{equation}
\mathrm{MSE}(\widehat{\mathrm{SM}}^{\mathrm{trig}}_{m}(\mathbf{x}, \mathbf{y})) = \frac{1}{m}\exp(\|\mathbf{x}\|^{2}+\|\mathbf{y}\|^{2}) \mathrm{Var}(\cos(\omega^{\top}\Delta)).     
\end{equation}
Using the fact that (see: Lemma 1 in \cite{ORF}; note that in that lemma they use notation: $z$ for what we denote as: $\|\Delta\|$):
\begin{equation}
\mathrm{Var}(\cos(\omega^{\top}\Delta))=\frac{1}{2}(1-\exp(-\|\Delta\|^{2}))^{2},    
\end{equation}
we obtain:
\begin{align}
\begin{split}
\mathrm{MSE}(\widehat{\mathrm{SM}}^{\mathrm{trig}}_{m}(\mathbf{x}, \mathbf{y})) = \frac{1}{2m}\exp(\|\mathbf{x}\|^{2}+\|\mathbf{y}\|^{2})(1-\exp(-\|\Delta\|^{2}))^{2} = \\
\frac{1}{2m} \exp(\|\mathbf{z}\|^{2})\mathrm{SM}^{-2}(\mathbf{x},\mathbf{y})(1-\exp(-\|\Delta\|^{2}))^{2},
\end{split}
\end{align}
which completes the first part of the proof.
To obtain the formula for: $\mathrm{MSE}(\widehat{\mathrm{SM}}^{\mathrm{+}}_{m}(\mathbf{x}, \mathbf{y}))$
notice first that:
\begin{equation}
\label{neat-fact}
\mathbb{E}_{\omega \sim \mathcal{N}(0, \mathbf{I}_{d})}[\exp(\omega^{\top}\mathbf{z})] = \exp(\frac{\|\mathbf{z}\|^{2}}{2}).    
\end{equation}
The above immediately follows from the fact that positive random feature maps provide unbiased estimation of the softmax-kernel, thus the following is true:
\begin{equation}
\mathrm{SM}(\mathbf{x}, \mathbf{y}) = \exp(-\frac{\|\mathbf{x}\|^{2}+\|\mathbf{y}\|^{2}}{2})\mathbb{E}_{\omega \sim \mathcal{N}(0, \mathbf{I}_{d})}[\exp(\omega^{\top}\mathbf{z})].    
\end{equation}

Therefore we obtain:
\begin{align}
\begin{split}
\mathrm{MSE}(\widehat{\mathrm{SM}}^{\mathrm{+}}_{m}(\mathbf{x}, \mathbf{y})) = \frac{1}{m} \exp(-(\|\mathbf{x}\|^{2} + \|\mathbf{y}\|^{2}))\mathrm{Var}(\exp(\omega^{\top}\mathbf{z})) = \\
\frac{1}{m} \exp(-(\|\mathbf{x}\|^{2} + \|\mathbf{y}\|^{2}))
\left(\mathbb{E}[\exp(2\omega^{\top}\mathbf{z})] - (\mathbb{E}[\exp(\omega^{\top}\mathbf{z})])^{2}\right) = \\ 
\frac{1}{m} \exp(-(\|\mathbf{x}\|^{2} + \|\mathbf{y}\|^{2}))
(\exp(2\|\mathbf{z}\|^{2}) - \exp(\mathbf{z}^{2})),
\end{split}  
\end{align}
where the last inequality follows from Equation \ref{neat-fact}.
Therefore we have:
\begin{align}
\begin{split}
\mathrm{MSE}(\widehat{\mathrm{SM}}^{\mathrm{+}}_{m}(\mathbf{x}, \mathbf{y})) = \frac{1}{m} \exp(-(\|\mathbf{x}\|^{2} + \|\mathbf{y}\|^{2})) \exp(\|\mathbf{z}\|^{2})(\exp(\|\mathbf{z}\|^{2}) - 1) = \\  
\frac{1}{m}\exp(\|\mathbf{z}\|^{2})\mathrm{SM}^{2}(\mathbf{x}, \mathbf{y})(1-\exp(-\|\mathbf{z}\|^{2})).
\end{split}
\end{align}
That completes the proof.
\end{proof}

\subsection{Proof of Lemma \ref{iid-lemma}}

\begin{proof}
Fix some $\theta > 0$. We have:
\begin{align}
\begin{split}
\mathbb{P}[\widehat{F}^{\mathrm{iid}}_{m}(\mathbf{z}) > a] = \mathbb{P}[e^{\theta m \widehat{F}^{\mathrm{iid}}_{m}(\mathbf{z})} > e^{\theta m a}]  
= \mathbb{P}[e^{\theta (X_{1}+...+X_{m})} > e^{\theta m a}],
\end{split}
\end{align}
where $X_{i}^{\mathrm{iid}} = g((\omega_{i}^{\mathrm{iid}})^{\top} \mathbf{z})$.
Thus, from Markov's inequality we get:
\begin{equation}
\mathbb{P}[\widehat{F}^{\mathrm{iid}}_{m}(\mathbf{z}) > a] \leq \frac{\mathbb{E}[e^{\theta (X_{1}^{\mathrm{iid}}+...+X_{m}^{\mathrm{iid}})}]}{e^{\theta ma}}.    
\end{equation}
Denote by $X$ a random variable with the same distribution as $X_{i}^{\mathrm{iid}}$ (clearly all $X_{i}^{\mathrm{iid}}$ have the same distribution since different $\omega_{i}^{\mathrm{iid}}$s are sampled from the same distribution $\Omega$).
Since different $\omega_{i}^{\mathrm{iid}}$s are independent, we conclude that different $X_{i}^{\mathrm{iid}}s$ are independent and thus we get:
\begin{equation}
\mathbb{P}[\widehat{F}^{\mathrm{iid}}_{m}(\mathbf{z}) > a] \leq 
\frac{\prod_{i=1}^{m} \mathbb{E}[e^{\theta X_{i}^{\mathrm{iid}}} ]}{e^{\theta ma}} = (\frac{\mathbb{E}[e^{\theta X}]}{e^{\theta a}})^{m}. 
\end{equation}
To obtain the tightest possible upper bound, we optimize over $\theta > 0$ and that completes the proof.
\end{proof}

\subsection{Proof of Theorem \ref{ort-theorem}}

Below we give the proof of Theorem \ref{ort-theorem}.
\begin{proof}
Note that by the analogous analysis to the one in the proof of Lemma \ref{iid-lemma}, we get:
\begin{align}
\begin{split}
\mathbb{P}[\widehat{F}^{\mathrm{ort}}_{m}(\mathbf{z})) > a] \leq   
\frac{\mathbb{E}[e^{\theta (X_{1}^{\mathrm{ort}}+...+X_{m}^{\mathrm{ort}})}]}{e^{\theta ma}},
\end{split}    
\end{align}
where we have:
$X_{i}^{\mathrm{ort}} = g((\omega_{i}^{\mathrm{ort}})^{\top}\mathbf{z})$.
We see that it suffices to show that for any $\theta > 0$ the following holds: 
$\mathbb{E}[e^{\theta (X_{1}^{\mathrm{ort}}+...+X_{m}^{\mathrm{ort}})}] < \mathbb{E}[e^{\theta (X_{1}^{\mathrm{iid}}+...+X_{m}^{\mathrm{iid}})}]$.
We have: 
\begin{align}
\begin{split}
\mathbb{E}[e^{\theta (X_{1}^{\mathrm{ort}}+...+X_{m}^{\mathrm{ort}})}] = \mathbb{E}[\sum_{j=0}^{\infty} \frac{(\theta \sum_{i=1}^{m} X_{i}^{\mathrm{ort}})^{j}}{j!}] 
= \mathbb{E}[\sum_{j=0}^{\infty}\frac{\theta^{j}}{j!}(\sum_{i=1}^{m}X^{\mathrm{ort}}_{i})^{j}]=\\
\sum_{j=0}^{\infty}\frac{\theta^{j}}{j!} \mathbb{E}[(\sum_{i=1}^{m} X^{\mathrm{ort}}_{i})^{j}]=
\sum_{j=0}^{\infty}\frac{\theta^{j}}{j!}
\mathbb{E}[\sum_{(j_{1},...,j_{m}) \in \mathcal{S}_{j}} c(j_{1},...,j_{m}) (X_{1}^{\mathrm{ort}})^{j_{1}} \cdot ... \cdot (X_{m}^{\mathrm{ort}})^{j_{m}}],
\end{split}
\end{align}
where $\mathcal{S}_{j} = \{(j_{1},...,j_{m}) \in \mathbb{N} \times ...\times \mathbb{N}:j_{1},...,j_{m} \geq 0, j_{1}+...+j_{m}=j\}$ and 
for some positive constants $c(j_{1},...,j_{m})$.

Thus we have:
\begin{equation}
\mathbb{E}[e^{\theta (X_{1}^{\mathrm{ort}}+...+X_{m}^{\mathrm{ort}})}] = \sum_{j=0}^{\infty} \frac{\theta^{j}}{j!} \sum_{(j_{1},...,j_{m}) \in \mathcal{S}_{j}} c(j_{1},...,j_{m}) \mathbb{E}[(X_{1}^{\mathrm{ort}})^{j_{1}} \cdot ... \cdot (X_{m}^{\mathrm{ort}})^{j_{m}}].  
\end{equation}

Similarly, we get:
\begin{equation}
\mathbb{E}[e^{\theta (X_{1}^{\mathrm{iid}}+...+X_{m}^{\mathrm{iid}})}] = \sum_{j=0}^{\infty} \frac{\theta^{j}}{j!} \sum_{(j_{1},...,j_{m}) \in \mathcal{S}_{j}} c(j_{1},...,j_{m}) \mathbb{E}[(X_{1}^{\mathrm{iid}})^{j_{1}} \cdot ... \cdot (X_{m}^{\mathrm{iid}})^{j_{m}}].    
\end{equation}

Therefore we get:
\begin{align}
\begin{split}
\Delta = \mathbb{E}[e^{\theta (X_{1}^{\mathrm{iid}}+...+X_{m}^{\mathrm{iid}})}] - \mathbb{E}[e^{\theta (X_{1}^{\mathrm{ort}}+...+X_{m}^{\mathrm{ort}})}] \\
=
\sum_{j=0}^{\infty} \frac{\theta^{j}}{j!} \sum_{(j_{1},...,j_{m}) \in \mathcal{S}_{j}} c(j_{1},...,j_{m}) \left(\mathbb{E}[(X_{1}^{\mathrm{iid}})^{j_{1}} \cdot ... \cdot (X_{m}^{\mathrm{iid}})^{j_{m}}] - \mathbb{E}[(X_{1}^{\mathrm{ort}})^{j_{1}} \cdot ... \cdot (X_{m}^{\mathrm{ort}})^{j_{m}}]\right)
\end{split}
\end{align}

% Since $\theta > 0$ and $c(j_{1},...,j_{m}) > 0$, % it suffices to show that:
% $\mathbb{E}[(X_{1}^{\mathrm{ort}})^{j_{1}} \cdot % ... \cdot (X_{m}^{\mathrm{ort}})^{j_{m}}] \leq % \mathbb{E}[(X_{1}^{\mathrm{iid}})^{j_{1}} \cdot ... % \cdot (X_{m}^{\mathrm{iid}})^{j_{m}}]$ for all % $j_{1},...,j_{m} \geq 0$ and furthermore, there % exist sequences $(j_{1},...,j_{m})$ for which the % inequality is strict.

Note first that using the fact that $f$ is entire, we can rewrite each $X_{i}^{\mathrm{ort}}$ as:
\begin{equation}
\label{x_ort_formula}
X_{i}^{\mathrm{ort}} = \sum_{s=0}^{\infty} a_{s}((\omega_{i}^{\mathrm{ort}})^{\top}\mathbf{z})^{s},
\end{equation}

where $f(x) = \sum_{s=0}^{\infty} a_{s}x^{s}$
and $a_{0},a_{1},... \geq 0$.
Similarly,
\begin{equation}
\label{x_iid_formula}
X_{i}^{\mathrm{iid}} = \sum_{s=0}^{\infty} a_{s}((\omega_{i}^{\mathrm{iid}})^{\top}\mathbf{z})^{s}.
\end{equation}

By plugging in the above formulae for $X_{i}^{\mathrm{ort}}$ and $X_{i}^{\mathrm{iid}}$ int the formula for $\Delta$ and expanding power-expressions, we obtain:
\begin{align}
\begin{split}
\Delta = \sum_{j=0}^{\infty} \frac{\theta^{j}}{j!} \sum_{(j_{1},...,j_{m}) \in \mathcal{S}_{j}} c(j_{1},...,j_{m}) \sum_{(d_{1},...,d_{m}) \in \mathcal{D}(j_{1},...,j_{m})} \widehat{\Delta}(d_{1},...,d_{m}),
\end{split}    
\end{align}
for some ordered subsets of indices (with potentially repeating entries) $\mathcal{D}(j_{1},...,j_{m})$ (exact formula for those can be given but we do not need it to complete the proof and since it is technical, it would unnecessarily complicate the proof so we skip it)
and $\widehat{\Delta}(d_{1},...,d_{m})$ defined as:
\begin{align}
\begin{split}
\label{imp-ineq}
\widehat{\Delta}(d_{1},...,d_{m}) = \mathbb{E}[((\omega_{1}^{\mathrm{iid}})^{\top}\mathbf{z})^{d_{1}} \cdot ... \cdot ((\omega_{m}^{\mathrm{iid}})^{\top}\mathbf{z})^{d_{m}}] - 
\mathbb{E}[((\omega_{1}^{\mathrm{ort}})^{\top}\mathbf{z})^{d_{1}} \cdot ... \cdot ((\omega_{m}^{\mathrm{ort}})^{\top}\mathbf{z})^{d_{m}}].
\end{split}
\end{align}

Our next goal is to re-write the formula for $\widehat{\Delta}(d_{1},...,d_{m})$. Denote:
\begin{equation}
Y = ((\omega_{1}^{\mathrm{ort}})^{\top}\mathbf{z})^{d_{1}} \cdot ... \cdot ((\omega_{m}^{\mathrm{ort}})^{\top}\mathbf{z})^{d_{m}}.    
\end{equation}

Observe that $Y$ has the same distribution as $Y^{\prime}$ defined as:

\begin{equation}
Y^{\prime} = (\mathbf{e}_{1}^{\top}\frac{\mathbf{g}}{\|\mathbf{g}\|_{2}}\|\mathbf{z}\|_{2})^{d_{1}} \cdot ... \cdot (\mathbf{e}_{m}^{\top}\frac{\mathbf{g}}{\|\mathbf{g}\|_{2}}\|\mathbf{z}\|_{2})^{d_{m}} \cdot
(\|\omega_{1}^{\mathrm{ort}}\|_{2})^{d_{1}} \cdot ... \cdot
(\|\omega_{m}^{\mathrm{ort}}\|_{2})^{d_{m}},
\end{equation}

where $\mathbf{g}$ is a Gaussian vector taken from the $\mathcal{N}(0,\mathbf{I}_{d})$ distribution, independently from: $\|\omega_{1}^{\mathrm{ort}}\|_{2},...,\|\omega_{m}^{\mathrm{ort}}\|_{2}$. 

This comes from the fact that for a fixed $\mathbf{z}$ one can think about the set:
$\frac{\omega_{1}^{\mathrm{ort}}}{\|\omega_{1}^{\mathrm{ort}}\|_{2}},...,\frac{\oomega_{m}^{\mathrm{ort}}}{\|\omega_{m}^{\mathrm{ort}}\|_{2}}$ as a random rotation of the system of $m$ canonical basis vectors: $\mathbf{e}_{1},...,\mathbf{e}_{m}$.
Thus instead of applying a random rotation to: $\mathbf{e}_{1},...,\mathbf{e}_{m}$, one can equivalently randomly rotate vector $\mathbf{z}$. Randomly rotated vector $\mathbf{z}$ has the same distribution as: $\frac{\mathbf{g}}{\|\mathbf{g}\|_{2}}\|\mathbf{z}\|_{2}$. 

%It remains to observe that the independence of $\mathbf{g}$ from %$\|\mathbf{w}_{1}^{\mathrm{ort}}\|_{2},...,\|\mathbf{w}_{m}^{\mathrm{%ort}}\|_{2}$ is implied by the fact that directions of vectors %$\mathbf{w} \sim \mathcal{D}$ are taken independently from their %lengths.

Now note that lengths of vectors $\omega_{1}^{\mathrm{ort}},...,\omega_{m}^{\mathrm{ort}}$ are chosen independently.

Therefore we obtain:
\begin{align}
\begin{split}
\mathbb{E}[((\omega_{1}^{\mathrm{ort}})^{\top}\mathbf{z})^{d_{1}} \cdot ... \cdot ((\omega_{m}^{\mathrm{ort}})^{\top}\mathbf{z})^{d_{m}}] = \mathbb{E}[(\|\omega_{1}^{\mathrm{ort}}\|_{2})^{d_{1}}] \cdot ... \cdot \mathbb{E}[(\|\omega_{m}^{\mathrm{ort}}\|_{2})^{d_{m}}] \cdot \\
\mathbb{E}[(\mathbf{e}_{1}^{\top}\mathbf{v})^{d_{1}} \cdot ... \cdot (\mathbf{e}_{m}^{\top}\mathbf{v})^{d_{m}}]
\|\mathbf{z}\|_{2}^{d_{1}+...+d_{m}},
\end{split}
\end{align}
where $\mathbf{v} \sim \frac{\mathbf{g}}{\|\mathbf{g}\|_{2}}$.

Denote $\mathbf{g}=(g_{1},...,g_{d})^{\top}$.
Thus we obtain:
\begin{align}
\begin{split}
\label{lhs}
\mathbb{E}[((\omega_{1}^{\mathrm{ort}})^{\top}\mathbf{z})^{d_{1}} \cdot ... \cdot ((\omega_{m}^{\mathrm{ort}})^{\top}\mathbf{z})^{d_{m}}] =  \mathbb{E}[(\|\omega_{1}^{\mathrm{ort}}\|_{2})^{d_{1}}] \cdot ... \cdot \mathbb{E}[(\|\omega_{m}^{\mathrm{ort}}\|_{2})^{d_{m}}] \cdot \\
\|\mathbf{z}\|_{2}^{d_{1}+...+d_{m}} 
\mathbb{E}[\frac{g_{1}^{d_{1} \cdot ... \cdot}g_{m}^{d_{m}}   }{\sqrt{g_{1}^{2}+...+g_{d}^{2}}^{d_{1}+...+d_{m}}}]
\end{split}
\end{align}

Now let us focus on the second expression from th eformula on $\widehat{\Delta}(d_{1},...,d_{m})$. We have:
\begin{align}
\begin{split}
\label{rhs}
\mathbb{E}[((\omega_{1}^{\mathrm{iid}})^{\top}\mathbf{z})^{d_{1}} \cdot ... \cdot ((\omega_{m}^{\mathrm{iid}})^{\top}\mathbf{z})^{d_{m}}] = \prod_{i=1}^{m} \mathbb{E}[((\omega_{i}^{\mathrm{iid}})^{\top}\mathbf{z})^{d_{i}}]   
= \\ \mathbb{E}[(\|\omega_{1}^{\mathrm{iid}}\|_{2})^{d_{1}}] \cdot ... \cdot \mathbb{E}[(\|\omega_{m}^{\mathrm{iid}}\|_{2})^{d_{m}}] \cdot \|\mathbf{z}\|_{2}^{d_{1}+...+d_{m}} \cdot \\
\prod_{i=1}^{m} \mathbb{E}[\frac{g_{i}^{d_{i}}}{\sqrt{g_{1}^{2}+...+g_{d}^{2}}^{d_{i}}}],
\end{split}
\end{align}

where the first equality comes from the fact that
different $\omega_{i}^{\mathrm{iid}}$s are independent and the second one is implied by the analogous analysis to the one conducted above.

We will need the following lemma:

\begin{lemma}
\label{useful-lemma}
For every $s \in \mathbb{N}_{+}$ such that $s \leq n$ and every $k_{1},...,k_{s} \in \mathbb{N}_{+}$ the following holds:
\begin{equation}
\mathbb{E}[\frac{g_{1}^{k_{1}} \cdot ... \cdot g_{s}^{k_{s}}}{\sqrt{g_{1}^{2}+...+g_{d}^{2}}^{k_{1}+...+k_{s}}}] = \frac{\prod_{i=1}^{s}\mathbb{E}[g_{i}^{k_{i}}]}{\mathbb{E}[\sqrt{g_{1}^{2}+...+g_{d}^{2}}^{k_{1}+...+k_{s}}]}.    
\end{equation}
\end{lemma}

\begin{proof}
Take $\mathbf{r} = \frac{\mathbf{g}}{\|\mathbf{g}\|_{2}}\|\tilde{\mathbf{g}}\|_{2}$, where $\tilde{\mathbf{g}}$ is an independent copy of $\mathbf{g}$. Note that $\mathbf{r} \sim \mathbf{g}$.
We have:
\begin{align}
\begin{split}
\mathbb{E}[r_{1}^{k_{1}}] \cdot ... \cdot     
\mathbb{E}[r_{s}^{k_{s}}] = 
\mathbb{E}[r_{1}^{k_{1}} \cdot ... \cdot r_{s}^{k_{s}}]
= \mathbb{E}[\frac{g_{1}^{k_{1}} \cdot ... \cdot g_{s}^{k_{s}}}{\sqrt{g_{1}^{2}+...+g_{d}^{2}}^{k_{1}+...+k_{s}}}] \\
\cdot \mathbb{E}[\|\tilde{\mathbf{g}}\|_{2}^{k_{1}+...+k_{s}}],
\end{split}    
\end{align}
where the first equality comes from the independence of different elements of $\mathbf{z}=(z_{1},...,z_{n})^{\top}$
and the second equality is implied by the fact that $\tilde{\mathbf{g}}$ is independent from $\mathbf{g}$.

Therefore we have:
\begin{equation}
 \mathbb{E}[\frac{g_{1}^{k_{1}} \cdot ... \cdot g_{s}^{k_{s}}}{\sqrt{g_{1}^{2}+...+g_{d}^{2}}^{k_{1}+...+k_{s}}}] = \frac{\mathbb{E}[r_{1}^{k_{1}}] \cdot ... \cdot     \mathbb{E}[r_{s}^{k_{s}}]}{\mathbb{E}[\|\tilde{\mathbf{g}}\|_{2}^{k_{1}+...+k_{s}}]}.   
\end{equation}
That completes the proof since $\mathbf{z} \sim \mathbf{g}$ and $\tilde{\mathbf{g}} \sim \mathbf{g}$.
\end{proof}

Note that by Lemma \ref{useful-lemma}, we can rewrite the right expression from the formula on 
$\widehat{\Delta}(d_1,..., d_m)$
as: 
\begin{equation}
\mathbb{E}[(\|\omega_{1}^{\mathrm{ort}}\|_{2})^{d_{1}}] \cdot ... \cdot \mathbb{E}[(\|\omega_{m}^{\mathrm{ort}}\|_{2})^{d_{m}}] \cdot \\
\|\mathbf{z}\|_{2}^{d_{1}+...+d_{m}}\frac{\prod_{i=1}^{m}\mathbb{E}[g_{i}^{d_{i}}]}{\mathbb{E}[\sqrt{g_{1}^{2}+...+g_{d}^{2}}^{d_{1}+...+d_{m}}]}.
\end{equation}
The left expression from the formula on 
$\widehat{\Delta}(d_1,..., d_m)$ can be rewritten as:
\begin{align}
\begin{split}
L(d_{1},...,d_{m}) = \mathbb{E}[(\|\omega_{1}^{\mathrm{iid}}\|_{2})^{d_{1}}] \cdot ... \cdot \mathbb{E}[(\|\omega_{m}^{\mathrm{iid}}\|_{2})^{d_{m}}] \cdot 
\|\mathbf{z}\|_{2}^{d_{1}+...+d_{m}} \\
\frac{\prod_{i=1}^{m}\mathbb{E}[g_{i}^{d_{i}}]}
{\mathbb{E}[\sqrt{g_{1}^{2}+...+g_{d}^{2}}^{d_{1}}] \cdot ...\cdot \mathbb{E}[\sqrt{g_{1}^{2}+...+g_{d}^{2}}^{d_{m}}]}.
\end{split}
\end{align}

Since marginal distributions of $\omega_{i}^{\mathrm{ort}}$ and $\omega_{i}^{\mathrm{iid}}$ are the same, we can rewrite $\widehat{\Delta}(d_{1},...,d_{n})$ as:
\begin{equation}
\widehat{\Delta}(d_{1},...,d_{m})=
L(d_{1},...,d_{m})(1 - \tau(d_{1},...,d_{m})),
\end{equation}
where $\tau(d_{1},...,d_{m})$ is defined as:
\begin{equation}
\tau(d_{1},...,d_{m}) = \frac{\mathbb{E}[\sqrt{g_{1}^{2}+...+g_{d}^{2}}^{d_{1}}] \cdot ...\cdot \mathbb{E}[\sqrt{g_{1}^{2}+...+g_{d}^{2}}^{d_{m}}]}
{\mathbb{E}[\sqrt{g_{1}^{2}+...+g_{d}^{2}}^{d_{1}+...+d_{m}}]}     
\end{equation}
We need now few observations regarding $\widehat{\Delta}(d_{1},...,d_{m})$.
Note firsr that since odd moments of the Gaussian scalar distribution $\mathcal{N}(0, 1)$ are zero, $\widehat{\Delta}(d_{1},...,d_{m})$ is zero if at least of of $d_{i}$ is odd. Furthermore, $\wideehat{\Delta(d_{1},...,d_{m})}$ is trivially zero if all but at most one $d_{i}$ are zero.

With our new notation, $\Delta$ can be rewritten as:
\begin{align}
\begin{split}
\Delta = \sum_{j=0}^{\infty} \frac{\theta^{j}}{j!} \sum_{(j_{1},...,j_{m}) \in \mathcal{S}_{j}} c(j_{1},...,j_{m}) \sum_{(d_{1},...,d_{m}) \in \mathcal{D}(j_{1},...,j_{m})} L(d_{1},...,d_{m})(1-\tau(d_{1},...,d_{m})),
\end{split}    
\end{align}

Note also that we have:
\begin{align}
\begin{split}
e^{\theta(X_{1}^{\mathrm{iid}}+...+X_{m}^{\mathrm{iid}})} = \sum_{j=0}^{\infty} \frac{\theta^{j}}{j!} \sum_{(j_{1},...,j_{m}) \in \mathcal{S}_{j}} c(j_{1},...,j_{m}) \sum_{(d_{1},...,d_{m}) \in \mathcal{D}(j_{1},...,j_{m})} L(d_{1},...,d_{m}).
\end{split}    
\end{align}

Therefore (see: our observations on $\widehat{\Delta}(d_{1},...,d_{m})$) to complete the proof it suffices to show that: $\tau(d_{1},...,d_{m}) \leq \frac{d}{d+2}$ if at least two: $d_{i}$, $d_{j}$ for $i \neq j$ are nonzero and all $d_{i}$ are even.
\begin{lemma}
\label{tau-lemma}
The following holds if for some $i \neq j$ we have: $d_{i}, d_{j} > 0$ and all $d_{i}$ are even:
\begin{equation}
\tau(d_{1},...,d_{m}) \leq \frac{d}{d+2}.    
\end{equation}
\end{lemma}
\begin{proof}
Note that $\tau(d_{1},...,d_{m})$ can bee rewritten as:
\begin{equation}
\label{multi-d}
\tau(d_{1},...,d_{m}) = \frac{\prod_{i=1}^{m} \mu_{d}(d_{i})}{\mu_{d}(\sum_{i=1}^{m} d_i)},    
\end{equation}
where $\mu_{d}(j)$ stands for the $j^{th}$ moment of the $\chi$-distribution with $d$ degrees of freedom.
Note that $\mu_{d}(j) = 2^{\frac{j}{2}}
\frac{\Gamma(\frac{d+j}{2})}{\Gamma(\frac{d}{2})}$,
where $\Gamma$ is the so-called \textit{Gamma-function}.

Using the fact that: $\Gamma(n) = (n-1)!$ and $\Gamma(n+\frac{1}{2})=\frac{(2n-1)!!}{2^{n}}\sqrt{\pi}$ for $n \in \mathbb{N}_{+}$, it is easy to see 
that for a fixed $d$, the RHS of the Equality \ref{multi-d} is maximized when $d_{i}=d_{j}=2$ and $d_{k}=0$ for some $i \neq j$ and $k \notin \{i,j\}$. Furthermore, straightforward calculations show that in that case the value of the RHS from Equality \ref{multi-d} is $\frac{d}{d+2}$. That completes the proof of the Lemma, and consequently, the proof of the entire Theorem.
\end{proof}

\end{proof}

%\begin{figure}[h!]
%\centering
%\includegraphics[scale=1.7]{universe.jpg}
%\caption{The Universe}
%\label{fig:univerise}
%\end{figure}

\subsection{Proof of Theorem \ref{var-theorem}}

\begin{proof}
We will use the notation from the proof of Theorem \ref{ort-theorem}.
Since both estimators: $\widehat{F}^{\mathrm{ort}}_{m}(\mathbf{z})$ and
$\widehat{F}^{\mathrm{iid}}_{m}(\mathbf{z})$ are unbiased, we have:
$\mathrm{MSE}(\widehat{F}^{\mathrm{ort}}_{m}(\mathbf{z})) = \mathrm{Var}(\widehat{F}^{\mathrm{ort}}_{m}(\mathbf{z}))$ and
$\mathrm{MSE}(\widehat{F}^{\mathrm{iid}}_{m}(\mathbf{z})) = \mathrm{Var}(\widehat{F}^{\mathrm{iid}}_{m}(\mathbf{z}))$.
We have:
\begin{align}
\begin{split}
\mathrm{Var}(\widehat{F}^{\mathrm{iid}}_{m}(\mathbf{z})) = 
\mathbb{E}[(\widehat{F}^{\mathrm{iid}}_{m}(\mathbf{z})-\mathbb{E}[\widehat{F}^{\mathrm{iid}}_{m}(\mathbf{z})])^{2}] =
\mathbb{E}[(\widehat{F}^{\mathrm{iid}}_{m}(\mathbf{z}))^{2}]-
F^{2}(\mathbf{z}).
\end{split}
\end{align}

Similarly,
\begin{align}
\begin{split}
\mathrm{Var}(\widehat{F}^{\mathrm{ort}}_{m}(\mathbf{z})) = 
\mathbb{E}[(\widehat{F}^{\mathrm{ort}}_{m}(\mathbf{z}))^{2}]-
F^{2}(\mathbf{z}).
\end{split}
\end{align}

We have: 
\begin{align}
\begin{split}
\mathbb{E}[(\widehat{F}^{\mathrm{iid}}_{m}(\mathbf{z}))^{2}]
= \frac{1}{m^{2}}\sum_{i=1}^{m}\mathbb{E}[(X_{i}^{\mathrm{iid}})^{2}]
+\frac{1}{m^{2}}\sum_{i \neq j} \mathbb{E}[X^{\mathrm{iid}}_{i}X^{\mathrm{iid}}_{j}].
\end{split}
\end{align}

Similarly, we get:
\begin{align}
\begin{split}
\mathbb{E}[(\widehat{F}^{\mathrm{ort}}_{m}(\mathbf{z}))^{2}]
= \frac{1}{m^{2}}\sum_{i=1}^{m}\mathbb{E}[(X_{i}^{\mathrm{ort}})^{2}]
+\frac{1}{m^{2}}\sum_{i \neq j} \mathbb{E}[X^{\mathrm{ort}}_{i}X^{\mathrm{ort}}_{j}].
\end{split}
\end{align}

Therefore, since marginal distributions of $X_{i}^{\mathrm{iid}}$ and $X_{i}^{\mathrm{ort}}$ are the same,  we have:
\begin{align}
\begin{split}
\label{mse-diff}
\mathrm{MSE}(\widehat{F}^{\mathrm{iid}}_{m}(\mathbf{z})) - \mathrm{MSE}(\widehat{F}^{\mathrm{ort}}_{m}(\mathbf{z})) = 
{m \choose 2} \cdot 2 \cdot \frac{1}{m^{2}}
(\mathbb{E}[X^{\mathrm{iid}}_{1}X^{\mathrm{iid}}_{2}]-
\mathbb{E}[X^{\mathrm{ort}}_{1}X^{\mathrm{ort}}_{2}])\\
=(1-\frac{1}{m})(\mathbb{E}[X^{\mathrm{iid}}_{1}X^{\mathrm{iid}}_{2}]-
\mathbb{E}[X^{\mathrm{ort}}_{1}X^{\mathrm{ort}}_{2}])
\end{split}
\end{align}
Plugging in the formula for $X^{\mathrm{ort}}_{i}$ and $X^{\mathrm{iid}}_{i}$ from Equation \ref{x_ort_formula} and Equation \ref{x_iid_formula}, and using our analysis from the proof of Theorem \ref{ort-theorem} we obtain:
\begin{align}
\begin{split}
 \mathrm{MSE}(\widehat{F}^{\mathrm{iid}}_{m}(\mathbf{z})) - \mathrm{MSE}(\widehat{F}^{\mathrm{ort}}_{m}(\mathbf{z})) =   
 (1-\frac{1}{m})\sum_{t,u=0}^{\infty}a_{t}a_{u}\|\mathbf{z}\|_{2}^{t+u}
 \mathbb{E}[\|\omega\|_{2}^{t}] \mathbb{E}[\|\omega\|_{2}^{u}] \cdot \\
\frac{\mathbb{E}[r^{t}]\mathbb{E}[r^{u}]}
{\mathbb{E}[\sqrt{g_{1}^{2}+...+g_{d}^{2}}^{t}]
\mathbb{E}[\sqrt{g_{1}^{2}+...+g_{d}^{2}}^{u}]}
(1-\tau(t, u)).
\end{split} 
\end{align}
for $\omega \sim \Omega$ and $r \sim \mathcal{N}(0, 1)$.
Thus, using Lemma \ref{tau-lemma}, we get:
\begin{align}
\begin{split}
 \mathrm{MSE}(\widehat{F}^{\mathrm{iid}}_{m}(\mathbf{z})) - \mathrm{MSE}(\widehat{F}^{\mathrm{ort}}_{m}(\mathbf{z})) \geq (1-\frac{1}{m})\frac{2}{d+2}\sum_{t,u=0}^{\infty}a_{t}a_{u}\|\mathbf{z}\|_{2}^{t+u}
 \mathbb{E}[\|\omega\|_{2}^{t}] \mathbb{E}[\|\omega\|_{2}^{u}] \cdot \\
\frac{\mathbb{E}[r^{t}]\mathbb{E}[r^{u}]}
{\mathbb{E}[\sqrt{g_{1}^{2}+...+g_{d}^{2}}^{t}]
\mathbb{E}[\sqrt{g_{1}^{2}+...+g_{d}^{2}}^{u}]}\\
= (1-\frac{1}{m})\frac{2}{d+2}   
\left(\sum_{t=0}^{\infty}a_{t}\|\mathbf{z}\|_{2}^{t}
 \mathbb{E}[\|\omega\|_{2}^{t}] \cdot 
\frac{\mathbb{E}[r^{t}]}
{\mathbb{E}[\sqrt{g_{1}^{2}+...+g_{d}^{2}}^{t}]}\right)^{2} = (1-\frac{1}{m})\frac{2}{d+2}F^{2}_{\Omega,g}(\mathbf{z}).
\end{split}    
\end{align}
That completes the proof.
\end{proof}
