# Supplementary material for: Hybrid Random Features
Source: arXiv:2110.04367 source file (2022-01-30)
Supplement: Supplementary file 4 [file experiment_appendix.tex]

\newpage

\subsection*{Comparisons in Different Angle Distributions}

Link: \href{https://docs.google.com/document/d/1OQs_qNgVaVQg9NnxOtaWxG1KCkbLI-DCGnskVc1pJBI/edit?usp=sharing}{Comparisons}

\subsection{Language Modeling Training Details}
For the Language Modeling tasks, we trained a $2$-layer LSTM with hidden size of $200$ and $650$ for the PennTree Bank and the WikiText2 datasets respectively. We tied the weights of the word embedding layer and the decoder layer~\cite{inan2017tying, press2017using}. Thus we can treat the masked language modeling problem as minimizing the cross entropy loss between the dot product of the model output and the class embedding obtained from the embedding layer with the target word. 
%%% Should I talk about the softmax temperatures here.
